# Supplementary material for: Learning Latent and Hierarchical Structures in Cognitive Diagnosis Models
Source: arXiv:2104.02143 source file (2022-04-01)
Supplement: Supplementary file 2 [file manuscript.wordcount.tex]

File: manuscript.tex
Encoding: utf8
Sum count: 11048
Words in text: 9924
Words in headers: 57
Words outside text (captions, etc.): 381
Number of headers: 18
Number of floats/tables/figures: 15
Number of math inlines: 660
Number of math displayed: 26
Subcounts:
  text+headers+captions (#headers/#floats/#inlines/#displayed)
  192+10+0 (2/0/2/0) _top_
  1045+1+0 (1/0/8/0) Section: Introduction
  53+2+0 (1/0/4/0) Section: Model Setup
  911+4+35 (1/2/88/5) Subsection: Hierarchical Cognitive Diagnosis Models
  286+6+0 (1/0/22/1) Subsection: CDMs as Restricted Latent Class Models
  0+3+0 (1/0/0/0) Section: Regularized Estimation Method
  1464+4+49 (1/2/85/7) Subsection: Motivation and Proposed Method
  1184+2+5 (1/1/158/3) Subsection: Theoretical Proporties
  0+2+0 (1/0/0/0) Section: Learning Algorithms
  494+3+9 (1/0/52/7) Subsection: Penalized EM Algorithm
  1054+5+53 (1/4/99/3) Subsection: Recover Latent Hierarchies and $Q$-matrix
  1397+2+121 (1/3/86/0) Section: Simulation Studies
  0+3+0 (1/0/0/0) Section: Real Data Analysis
  800+4+92 (1/2/33/0) Subsection: Analysis of ECPE Data
  461+4+17 (1/1/20/0) Subsection: Analysis of PISA Data
  545+1+0 (1/0/3/0) Section: Discussion
  38+1+0 (1/0/0/0) Section: Acknowledgments
